# Supplementary material for: Optimal superconductivity in twisted bilayer WSe$_2$ where the Van Hove singularity crosses half-filling
Source: arXiv:2510.21384 ancillary file (2025-10-24)
Supplement: Supplementary file 1 [file Supplementary_Materials.pdf]

# Supplemental Materials for Optimal superconductivity in twisted bilayer $WSe_2$ where the Van Hove singularity crosses half-filling

Michał Zegrodnik,* Waseem Akbar, and Andrzej Biborski

*Academic Centre for Materials and Nanotechnology,*

*AGH University of Krakow, Al. Mickiewicza 30, 30-059 Krakow, Poland*

Louk Rademaker

*Department of Theoretical Physics, University of Geneva, CH-1211 Geneva, Switzerland and*

*Institute-Lorentz for Theoretical Physics, Leiden University,*

*PO Box 9506, Leiden, NL-2300, The Netherlands*

## I. GENERAL FEATURES OF THE MODEL

Here we provide details related with the applied theoretical approach based on the moiré $t$-$J$-$U$ model supplemented with the intersite Coulomb repulsion term. As a reminder below we show the complete form of the Hamiltonian from the main text of our analysis

$$\begin{aligned}\hat{H} = t\sum_{\langle ij\rangle\sigma} e^{i\sigma\nu_{ij}\phi}\,\hat{c}^{\dagger}_{i\sigma}\hat{c}_{j\sigma} \\ + J\sum_{\langle ij\rangle}{}' \left(\hat{S}^z_i\hat{S}^z_j + \frac{1}{2}e^{i2\nu_{ij}\phi}\hat{S}^+_i\hat{S}^-_j + \frac{1}{2}e^{-i2\nu_{ij}\phi}\hat{S}^-_i\hat{S}^+_j\right) \\ + U\sum_i \hat{n}_{i\uparrow}\hat{n}_{j\downarrow} + V\sum_{\langle ij\rangle}{}' \hat{n}_i\hat{n}_j,\end{aligned} \tag{S1}$$

where $\sigma = \pm 1$ represents spin up/down, $\hat{c}^{\dagger}_{i\sigma}$ and $\hat{c}_{i\sigma}$ are the creation and anihilation operators for electron with spin $\sigma$ at site $i$ of a triangular lattice, $\langle i, j\rangle$ correspond to nearest neighbors, $S^z_i$, $S^+_i$, $S^-_i$ are the spin-$\frac{1}{2}$ $z$ component, rising and lowering operators, respectively, $\hat{n}_{i\sigma}$ is the occupancy operator and $\hat{n}_i = \sum_\sigma \hat{n}_{i\sigma}$. The primed summation means that each bond between the lattice sites appears only once. The subsequent terms of the above Hamiltonian correspond to electron hopping, intersite exchange interaction, as well as intra-/inter-site Coulomb repulsion. The phase factors of the exponents have an alternating sign introduced by $\nu_{ij} = \pm 1$, which depends on the bond direction (cf. Fig. S1).

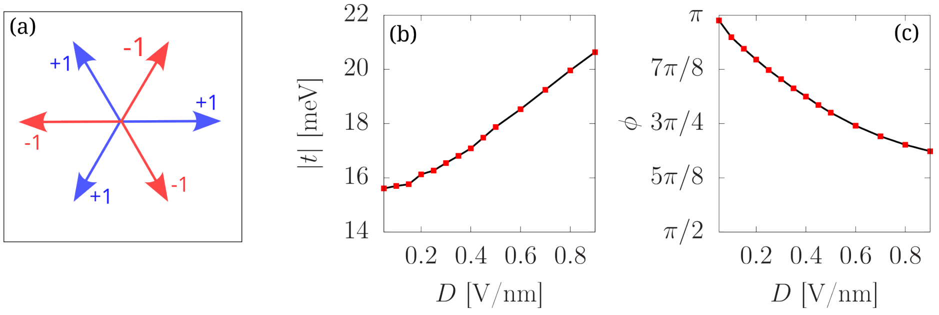


FIG. S1. (a) Values of the direction dependent factor ($\nu_{ij}$) appearing in the hoppings of the effective single-band model. (b) Absolute value of the hoppings as a function of the displacement field. (c) Phase factor $\phi$ as a function of displacement field, $D$. The data visualized by Figs. (b) and (c) have been calculated in Ref. [1] for the twist angle of $\theta = 5.08°$ and are used in our analysis.

---

* michal.zegrodnik@agh.edu.pl

It should be noted that, due to inversion symmetry breaking in transition-metal dichalcogenide quasi-two-dimentional systems, there is a significant valley-dependent spin-orbit coupling, which acts like an effective Zeeman field with opposite out-of-plane directions. Such Ising-type spin-orbit coupling results in spin-momentum locking perpendicular to the two-dimensional crystal near the $K$ and $K'$ valleys (so-called spin-valley locking) [2, 3]. The effect also appears in twisted TMD-based structures and can be tuned by experimentally controllable factors such as the displacement field ($D$), which is the bias voltage across the layered structure [4, 5]. This is one of the characteristic features which distinguishes the TMD-based moiré systems from those graphene-based.

Here we follow Refs. 1 and 4 where it has been shown that the effect of the Ising type spin-orbit coupling can be taken into account in an effective single-band picture of twisted $WSe_2$ bilayer by spin- and direction-dependent complex hoppings. As one can see, from Eq. (S1) and Fig. S1(a) the complex phase of the hoppings has opposite signs corresponding to the opposite hopping direction and opposite spin orientation. In principle, this leads to two separate Fermi surfaces corresponding to two values of the spin-valley degree of freedom, $\tau = 1$ for $(K, \uparrow)$ and $\tau = -1$ for $(K', \downarrow)$. As a result of the Ising-type spin orbit coupling the symmetry of the system is reduced from $C_6$ to $C_3$. In such a picture, the effect of the displacement field is taken into account via the absolute value of the hoppings ($t$) and the phase factor ($\phi$), which are $D$-dependent [cf. Fig. S1 (b) and (c)]. As presented in Fig. S2 by increasing the displacement field one enhances the Fermi surface spin splitting as well as changes the position of the Van Hove singularity from higher to lower band fillings. The $D$-dependant phase factor $\phi$ plays the major role in this effect. For very low displacement fields where $\phi \approx \pi$ the hopping parameters are nearly real numbers, meaning that the difference between the spin-up and spin-down Fermi surfaces should be minor, as seen in (f). In such a situation, the spin splitting is almost vanishing and the system is nearly $C_6$ symmetric. However, by increasing the displacement field the phase factor moves away from $\phi \approx \pi$ and spin-dependent imaginary part of the hoppings is increased, which enhances the Fermi surface spin splitting leading to a clear $C_3$ symmetry realized by the system.

Another visible effect of the displacement field and the Ising-type spin-orbit coupling is that by keeping constant band filling and increasing $D$ a transition occurs from electron-like (closed) to hole-like (opened) Fermi surfaces for some critical value of $D \approx 0.3 - 0.35$ V/nm. This transition corresponds to the Van Hove singularity passing through the Fermi energy

with increasing $D$. It results from the fact that the Van Hove singularity corresponds to a saddle point in the electronic structure, which connects the electron-like and hole-like Fermi surfaces, which is a characteristic feature of two-dimensional systems.

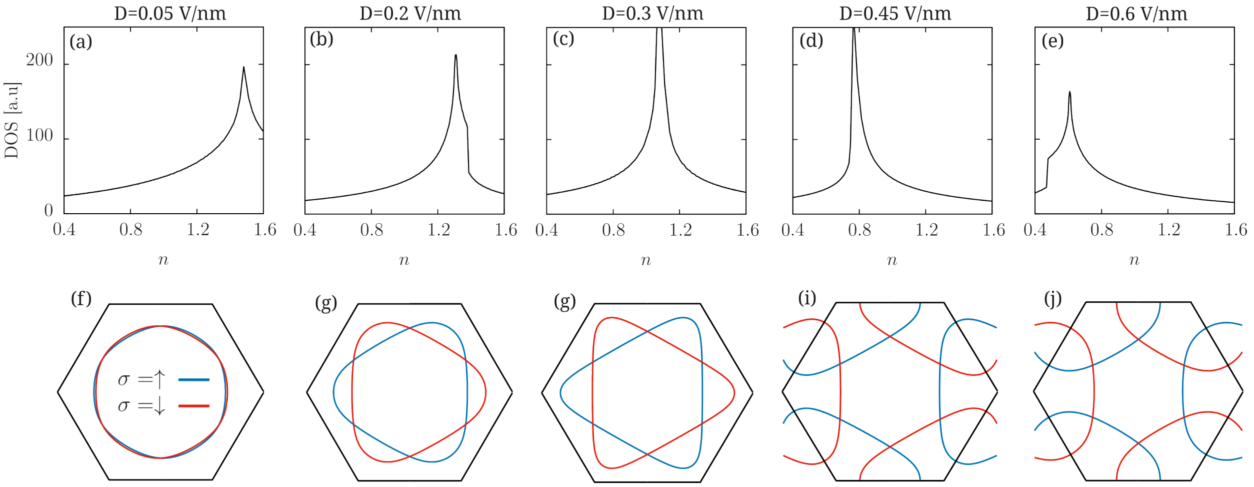


FIG. S2. (a-e) Density of states at the Fermi energy as a function of band filling for five different values of displacement field (provided in the figure). (f-j) the spin-up (blue) and spin-down (red) Fermi surfaces at half-filling corresponding to the subsequent values of the displacement fields provided in (a-e), respectively.

It should be noted that recently both the Hubbard and $t$-$J$ models have been discussed in the context of $tWSe_2$ [4, 6–10]. Here we use a slightly different approach in which both $U$- and $J$- terms are taken into account explicitly. Few methodological remarks related to the model itself are in place here. Namely, starting from the Hubbard model and assuming a large $U$ limit, the double occupancies are projected out, and the kinetic exchange term emerges resulting from virtual double occupancies leading to the $t$-$J$ model. On the other hand, in the limit of weak onsite Coulomb repulsion, double occupancies are allowed even close to half-filling, but the effect of kinetic exchange is no longer operative. The $t$-$J$-$U$ model should be considered as an effective approach dedicated to the situation when the $U$ value is in between the two limiting situations. If $U$ is substantial and not infinite, the double occupancies are small but non-zero, therefore the $U$ term should be present in the Hamiltonian. At the same time, the spin-spin kinetic exchange interaction already starts to develop. In order to explicitly take into account both effects, the $t$-$J$-$U$ model is used. Within the Gutzwiller approximation applied here, the effect of onsite correlations induced

by $U$ is taken into account via the variational wave function. However, the effect of spin-spin superexchange is captured by the $\sim J$ term. Additionally, we supplement the model with a $V$ term to take into account the effect of longer-range Coulomb repulsion.

The $t$-$J$-$U$ model has been proposed already some time ago and discussed in the context of general properties of correlated electron systems [11–15]. The concept is very much related to the so-called Gossamer superconductivity introduced by Laughlin [16] and discussed by F. C. Zhang [17]. It has also been shown that the approach based on the $t$-$J$-$U$ model allows to reproduce selected fundamental properties of the cuprates in a quantitative manner [18].

## II. THE VARIATIONAL WAVE FUNCTION

### A. The Gutzwiller-type wave function and the effective Hamiltonian

Since we are most interested in the moderately correlated ($U \approx W$) regime, we apply the variational wave function of Gutzwiller type which allows to take into account the electron-electron interactions. The considered variational wave function has the following form

$$|\Psi_G\rangle = \hat{P}|\Psi_0\rangle, \tag{S2}$$

where $|\Psi_0\rangle$ is the uncorrelated (mean-field) state and $\hat{P}$ is the correlation operator

$$\hat{P} = \prod_i \hat{P}_i = \prod_i \sum_\Gamma \lambda_{i,\Gamma} |\Gamma\rangle_{i\,i}\langle\Gamma|, \tag{S3}$$

where $i$ runs over all the lattice sites, $|\Gamma\rangle$ corresponds to the local basis $|\Gamma\rangle \in \{|\emptyset\rangle, |\uparrow\rangle, |\downarrow\rangle, |\uparrow\downarrow\rangle\}$, and $\lambda_{i,\Gamma}$ are the variational parameters. As shown by Bünemann et al., one can impose an additional condition to the correlation operator, in order to reduce the complexity of the numerical calculations [19], i.e.,

$$\hat{P}_i^2 = 1 + x\hat{d}_i^{HF}, \tag{S4}$$

where $\hat{d}_i^{HF} = \hat{n}_{i\uparrow}^{HF}\hat{n}_{i\downarrow}^{HF}$, $\hat{n}_{i\sigma}^{HF} = \hat{n}_{i\sigma} - n_{i\sigma}$, with $n_{i\sigma} = \langle\Psi_0|\hat{n}_{i\sigma}|\Psi_0\rangle$, and $x$ is yet another variational parameter. By using Eqs. (S3) and (S4) one can easily show that

$$\begin{aligned}
\lambda_{\uparrow\downarrow}^2 &= 1 + x(1-n_s)^2, \\
\lambda_s^2 &= 1 - xn_s(1-n_s), \\
\lambda_\emptyset^2 &= 1 + xn_s^2,
\end{aligned} \tag{S5}$$

where for simplicity we have assumed a homogeneous system with no magnetic or charge ordering. Hence, $\lambda_{i,\uparrow\downarrow} \equiv \lambda_{\uparrow\downarrow}$, $\lambda_{i,\uparrow} = \lambda_{i,\downarrow} \equiv \lambda_s$, $\lambda_{i,\emptyset} \equiv \lambda_\emptyset$, and $n_{i\uparrow} = n_{i\downarrow} \equiv n_s$. Via Eqs. (S5), the parameters $\lambda_{\uparrow\downarrow}$, $\lambda_s$, and $\lambda_\emptyset$ which correspond to doubly occupied, singly occupied, and empty lattice sites are all functions of the average number of particles in the system per site per spin and the variational parameter $x$. As a result, we are left with only one variational parameter, $x$.

In order to obtain the formula for the expectation value of our hamiltonian

$$E_G = \frac{\langle \Psi_G | \hat{H} | \Psi_G \rangle}{\langle \Psi_G | \Psi_G \rangle} = \langle \hat{H} \rangle_G, \tag{S6}$$

we apply the diagrammatic expansion of the Gutzwiller wave function (DE-GWF) [20] in the zeroth order which is equivalent to the *Statistically consistent Gutzwiller Approximation* (SGA) [15]. As a result, one can obtain the explicit form of all the energy contributions to $E_G$ resulting from subsequent terms appearing in Eq. (S1)

$$\begin{aligned}
E_0 &= \sum_{ij} q^2 t_{ij\sigma} \langle \hat{c}^\dagger_{i\sigma} \hat{c}_{j\sigma} \rangle_0, \\
E_J &= \lambda_s^4 J \sum_{\langle ij \rangle}{}' \left( \frac{1}{2} \sum_{\sigma} e^{i\sigma 2\phi_{ij}} \langle \hat{c}^\dagger_{i\sigma} \hat{c}_{i\bar{\sigma}} \hat{c}^\dagger_{j\bar{\sigma}} \hat{c}_{j\sigma} \rangle_0 + \frac{1}{4} \sum_{\sigma\sigma'} \sigma\sigma' \big( \langle \hat{n}_{i\sigma} \hat{n}_{j\sigma'} \rangle_0 - n_s^2 \big) \right), \\
E_U &= \lambda_{\uparrow\downarrow}^2 U \sum_i \langle \hat{n}_{i\uparrow} \hat{n}_{i\downarrow} \rangle_0, \\
E_V &= V \sum_{\langle ij \rangle}{}' \big( g_v^2 \langle \hat{n}_i \hat{n}_j \rangle_0 - (1 - g_v^2) n_s^2 \big),
\end{aligned} \tag{S7}$$

where $q = \lambda_s \big( \lambda_d n_s + \lambda_\emptyset (1 - n_s) \big)$, $g_v = (1 - (2 - \lambda_{\uparrow\downarrow}) n_s)/(1 - n_s)$, and $\langle \hat{o} \rangle_0$ stands for the expectation value of the $\hat{o}$ operator in the state $|\psi\rangle_0$. As one can see, the expectation value of a given energy term in the correlated state, $|\Psi_G\rangle$, can be expressed in terms of the expectation values in the unorrelated state, $|\Psi_0\rangle$. However, factors $q^2$, $\lambda_s^4$, $\lambda_{\uparrow\downarrow}^2$, and $g_v^2$ renormalize the hopping, exchange interactions $J$, onsite Coulomb repulsion $U$, and intersite Coulomb repulsion $V$, respectively. All the operator terms in Eqs. (S7) can be decomposed by applying the Wick's theorem. Hence, the obtained $E_G$ becomes a function of $x$, $n_s$ as well as the electron hopping and Cooper pairing mean field parameters,

$$P_{ij\sigma} = \langle \hat{c}^\dagger_{i\sigma} \hat{c}_{j\sigma} \rangle_0, \quad S_{ij}^{\sigma\sigma'} = \langle \hat{c}_{i\sigma} \hat{c}_{j\sigma'} \rangle_0, \tag{S8}$$

respectively. It should be noted that one can also calculate the corresponding quantities in

the correlated state which take the form

$$\begin{aligned}\Lambda_{ij\sigma} &= \langle \hat{c}^{\dagger}_{i\sigma}\hat{c}_{j\sigma}\rangle_G = q^2\langle \hat{c}^{\dagger}_{i\sigma}\hat{c}_{j\sigma}\rangle_0,\\ \Delta^{\sigma\sigma'}_{ij} &= \langle \hat{c}_{i\sigma}\hat{c}_{j\sigma'}\rangle_G = q^2\langle \hat{c}_{i\sigma}\hat{c}_{j\sigma'}\rangle_0.\end{aligned} \tag{S9}$$

The Gutzwiller projection does not change the number of particles ($\langle \hat{n}_{i\sigma}\rangle_G = \langle \hat{n}_{i\sigma}\rangle_0$), due to the fact that we are using the zeroth-order expansion of the Gutzwiller wave function and do not consider the standard on-site *s-wave* pairing scenario.

In order to determine the values of the mean fields given by Eqs. (S8), we apply the Effective Hamiltonian Scheme which is based on the minimization condition of the ground state energy [21]. In the considered case, the resulting form of the effective Hamiltonian is the following

$$\begin{aligned}\hat{\mathcal{H}}_{\text{eff}} = &\sum_{ij\sigma}\tilde{t}_{ij\sigma}\hat{c}^{\dagger}_{i\sigma}\hat{c}_{j\sigma} - \tilde{\mu}\sum_{i\sigma}\hat{n}_{i\sigma}\\ &+ {\sum_{\langle ij\rangle\sigma}}' \big((\tilde{\Delta}_{ij\sigma\bar{\sigma}})^*\hat{c}_{j\sigma}\hat{c}_{i\bar{\sigma}} + h.c.\big),\end{aligned} \tag{S10}$$

where the effective hopping, effective chemical potential, and effective superconducting gap parameters are defined through the corresponding relations

$$\tilde{t}_{ij\sigma} \equiv \frac{\partial\mathcal{F}}{\partial P_{ij\sigma}}, \quad (\tilde{\Delta}_{ij\sigma\bar{\sigma}})^* \equiv \frac{\partial\mathcal{F}}{\partial S^{\sigma\bar{\sigma}}_{ji}}, \quad \tilde{\mu} \equiv -\frac{\partial\mathcal{F}}{\partial n_s}, \tag{S11}$$

where $\mathcal{F} = E_G - 2\mu_G n_s$ with $\mu_G$ being the chemical potential determined in the correlated state.

After the transformation to the $\mathbf{k}$ space, one obtains

$$\begin{aligned}\hat{\mathcal{H}}_{\text{eff}} = &\sum_{\mathbf{k}\sigma}\begin{pmatrix}\hat{c}^{\dagger}_{\mathbf{k}\sigma} & \hat{c}_{-\mathbf{k}\bar{\sigma}}\end{pmatrix}\begin{pmatrix}\tilde{\epsilon}_{\mathbf{k}\sigma} - \tilde{\mu} & \tilde{\Delta}_{\mathbf{k}\bar{\sigma}\sigma}\\ (\tilde{\Delta}_{\mathbf{k}\bar{\sigma}\sigma})^* & -\tilde{\epsilon}_{\mathbf{k}\sigma} + \tilde{\mu}\end{pmatrix}\begin{pmatrix}\hat{c}_{\mathbf{k}\sigma}\\ \hat{c}^{\dagger}_{-\mathbf{k}\bar{\sigma}}\end{pmatrix}\\ &+ \sum_{\mathbf{k}\sigma}(\tilde{\epsilon}_{\mathbf{k}\sigma} - \tilde{\mu}),\end{aligned} \tag{S12}$$

where $\bar{\sigma} = -\sigma$ and

$$\begin{aligned}\tilde{\epsilon}_{\mathbf{k}\sigma} &= \sum_{i(j)}\tilde{t}_{ij}e^{ik(\mathbf{R}_i - \mathbf{R}_j)}\\ \tilde{\Delta}_{\mathbf{k}\bar{\sigma}\sigma} &= \sum_{i(j)}\tilde{\Delta}_{ji\sigma\bar{\sigma}}e^{ik(\mathbf{R}_j - \mathbf{R}_i)},\end{aligned} \tag{S13}$$

where we have used the time reversal symmetry condition ($\tilde{\epsilon}_{\mathbf{k}\sigma} = \tilde{\epsilon}_{-\mathbf{k}\bar{\sigma}}$) and $i$ index runs over the nearest-neighbor lattice sites of site $j$. The $\mathbf{R}_i$ and $\mathbf{R}_j$ vectors determine the positions of $i$ and $j$ lattice sites, respectively.

The resulting quasiparticle dispersion relations are the following

$$\lambda_{\mathbf{k}\sigma} = \pm\sqrt{(\tilde{\epsilon}_{\mathbf{k}\sigma} - \tilde{\mu})^2 + |\tilde{\Delta}_{\mathbf{k}\bar{\sigma}\sigma}|^2}. \tag{S14}$$

As one can see from the above equation, the SC gap $\tilde{\Delta}_{\mathbf{k}\downarrow\uparrow}$ ($\tilde{\Delta}_{\mathbf{k}\uparrow\downarrow}$) opens up at the spin up (spin down) Fermi surface. Next, we transform $\tilde{\Delta}_{\mathbf{k}\downarrow\uparrow}$ and $\tilde{\Delta}_{\mathbf{k}\uparrow\downarrow}$ into the singlet and triplet components as follows

$$\begin{aligned} \tilde{\Delta}^s_{\mathbf{k}} &= \frac{1}{\sqrt{2}}\big(\tilde{\Delta}_{\mathbf{k}\uparrow\downarrow} - \tilde{\Delta}_{\mathbf{k}\downarrow\uparrow}\big), \\ \tilde{\Delta}^t_{\mathbf{k}} &= \frac{1}{\sqrt{2}}\big(\tilde{\Delta}_{\mathbf{k}\uparrow\downarrow} + \tilde{\Delta}_{\mathbf{k}\downarrow\uparrow}\big), \end{aligned} \tag{S15}$$

which we can use to rewrite the expressions for the eigenvalues

$$\lambda_{\mathbf{k}\sigma} = \pm\sqrt{(\tilde{\epsilon}_{\mathbf{k}\sigma} - \tilde{\mu})^2 + \frac{1}{2}|\tilde{\Delta}^t_{\mathbf{k}} - \sigma\tilde{\Delta}^s_{\mathbf{k}}|^2}. \tag{S16}$$

As one can see from above, for the singlet-triplet mixed paired state, one can have different SC gaps opening at the spin-up and spin-down Fermi surfaces.

The self-consistent equations for the mean field parameters can be derived in a standard manner by applying the Bogolubov-de Gennes approach to the effective Hamiltonian in $\mathbf{k}$-space with the correlation effects taken into account via the renormalization factors. By solving the set of self-consistent equations numerically, we determine the hopping and pairing amplitudes to all the six nearest neighbors. Then, to obtain their correlated state counterparts, we use Eqs. (S9). It should be noted that the procedure for solving the self-consistent equations must be coupled with the minimization of the total energy of the system with respect to the variational parameter $x$, which then determines all the parameters $\lambda$ that appear in the correlated state $|\Psi_G\rangle$ by Eqs. (S5). In practice, this can be done by supplementing the set of self-consistent equations with the following

$$\frac{\partial E_G}{\partial x} = 0, \tag{S17}$$

where in our case the analytical derivative is replaced by a numerical one.

## B. The paired state

Note that the unprojected wave function already contains the superconducting order parameter defined by Eq. (S8). However, we do not impose the appearance of pairing on

the level of the wave function itself. Instead, we allow for the anomalous expectation values $S_{ij}^{\sigma\bar{\sigma}}$ to be non-zero during our numerical procedure. Also, we do not limit ourselves to one specific symmetry of the SC gap. Instead, we consider all possible pairing symmetries that are allowed for the case of triangular lattice within the nearest neighbor real-space pairing scenario. This requires solving the set of self-consistent equations for all the six complex nearest-neighbor gap amplitudes without any additional constraints. Moreover, we allow for pure spin-singlet pairing ($S_{ij}^{\uparrow\downarrow} = -S_{ij}^{\downarrow\uparrow}$), pure spin-triplet pairing ($S_{ij}^{\uparrow\downarrow} = S_{ij}^{\downarrow\uparrow}$), as well as their mixture ($|S_{ij}^{\uparrow\downarrow}| \neq |S_{ij}^{\downarrow\uparrow}|$). At the same time, we neglect the possibility of triplet $S^z = \pm 1$ pairing due to the fact that those pairing channels lead to a Fermi wave vector mismatch, which is detrimental when it comes to the formation of the superconducting state.

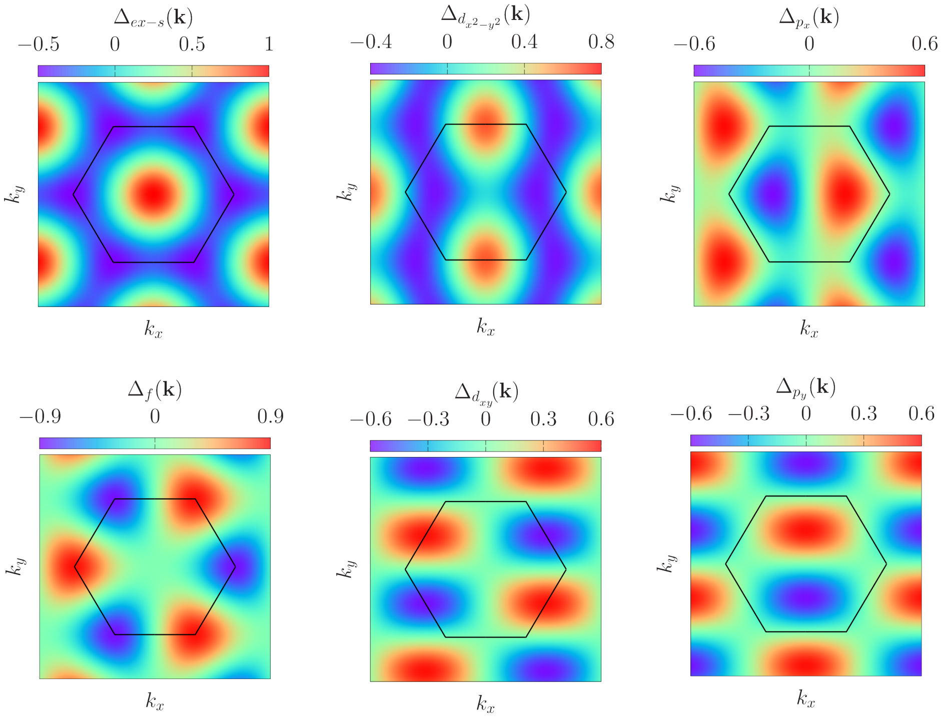


FIG. S3. The **k**-dependent SC gaps corresponding to the six symmetries which appear as real and imaginary parts of the pairing channels listed in Table I. The Brillouin zone is marked by black solid line. The presented distributions have been obtained by setting particular symmetry resolved factors to 1 and all the others to 0.

After we determine all the correlated SC amplitudes $\Delta_{ij}^{\bar{\sigma}\sigma}$ to the nearest neighbors, we transform them into the so-called symmetry resolved gap amplitudes in order to identify the symmetry of the resultant paired state. The symmetry-resolved pairing amplitudes are

| M | p | gap symmetry | parity | spin state |
|---|---|---|---|---|
| 0 | 0 | extended $s$ | even | singlet |
| 1 | 1 | $p_x + i\, p_y$ | odd | triplet |
| 2 | 0 | $d_{x^2-y^2} + i\, d_{xy}$ | even | singlet |
| 3 | 1 | $f$ | odd | triplet |
| 4 | 0 | $d_{x^2-y^2} - i\, d_{xy}$ | even | singlet |
| 5 | 1 | $p_x - i\, p_y$ | odd | triplet |

TABLE I. The six symmetries of the superconducting gap together with their parities and Cooper pair spin state. The symmetry factor, $M$, and the corresponding values of the parity factor $p$ are provided in the first and the second column, respectively [cf. Eq. (S18)].

defined by the following equation

$$\Delta^{\sigma\bar{\sigma}}_{M,p} = \frac{i^p}{6}\sum_{i(j)} e^{-iM\theta_{ji}}\Delta^{\sigma\bar{\sigma}}_{ji}, \tag{S18}$$

where the summation runs over the six nearest-neighbor lattice sites $j$ surrounding site $i$, and $\theta_{ji}$ are the angles $\{0,\ \pi/3,\ 2\pi/3,\ \pi,\ 4\pi/3,\ 5\pi/3\}$ between the positive half-$x$ axis and the $\mathbf{R}_{ji} = \mathbf{R}_j - \mathbf{R}_i$ vector. $M$ is the symmetry factor, which takes integer values and $p = 0$ for even-parities, and $p = 1$ for odd parities (cf. Table I).

Finally, we can write down the expressions for the real-space singlet and triplet gap amplitudes in the correlated state

$$\begin{aligned}\Delta^{s}_{M,p} &= (\Delta^{\uparrow\downarrow}_{M,p} - \Delta^{\downarrow\uparrow}_{M,p})/\sqrt{2},\\ \Delta^{t}_{M,p} &= (\Delta^{\uparrow\downarrow}_{M,p} + \Delta^{\downarrow\uparrow}_{M,p})/\sqrt{2}.\end{aligned} \tag{S19}$$

For the sake of clarity, in the main text of the paper, we use the symmetry names ($p \pm ip$, $d \pm id$, $f$ etc.) in the subscripts of the symmetry resolved superconducting gaps instead of the values of the $M$ and $p$ factors.

In Fig. S3 we show the six gap symmetries in reciprocal space, which appear as real and imaginary parts of the pairing channels listed in Table I. As one can see, the absolute values of the *extended s-wave* and *f-wave* SC gap is $C_6$ symmetric; hence those two appear as independent pairing channels possible for the triangular lattice. However, the remaining

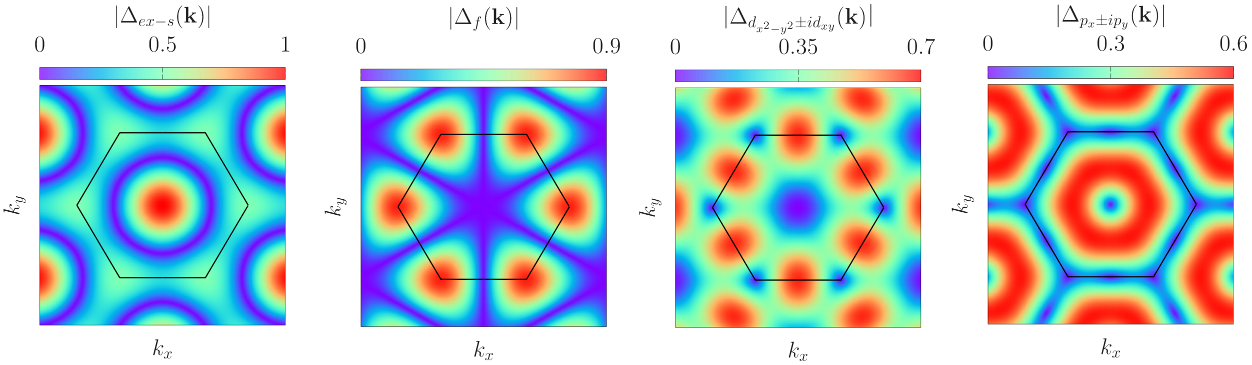


FIG. S4. The absolute value of the **k**-dependent SC gaps corresponding to the six pairing channels listed in Table I. The Brillouin zone is marked by black solid line. The presented distributions have been obtained by setting particular symmetry resolved factors to 1 and all the others to 0.

$d_{x^2-y2}$, $d_{xy}$, $d_{p_x}$, and $d_{p_y}$ are not C$_6$ symmetric; therefore, those create combinations $d_{x^2-y2} \pm id_{xy}$ and $p_x \pm ip_y$ which result in conserved symmetry of the lattice (cf. Fig. S4). It should be noted that, despite the fact that the lattice itself fulfills the mentioned C$_6$ symmetry, the Hamiltonian does not due to the spin-valley locking, which is taken into account via spin- and direction-dependent hoppings. Those lead to reduction of the symmetry to C$_3$ which has further consequences for the pairing symmetry as we show in the next section.

### C. Influence of spin-valley locking on the paired state

To show how the Ising-type spin orbit coupling and the resulting spin-valley locking influence the superconducting phase, we consider two representative situations at half-filling ($n = 1$). For the first one, there is no spin-valley locking, hence, we take a single particle term composed of purely real nearest-neighbor hoppings on a triangular lattice. For this case to induce the superconducting state at $n = 1$ we need to completely suppress the $V$ term; therefore, we have carried out calculations for the case of $t$-$J$-$U$ model just to analyze the gap symmetry. In this case the stable paired state corresponds to the $d \pm id$ symmetry (two degenerate solutions). The corresponding **k**-dependent SC gap is provided in Fig. S5(a) together with the normal-state Fermi surface. In the absence of SOC the system is C$_6$ symmetric and the spin-up and spin-down Fermi surfaces are identical (there is no spin-valley locking). As a result, the pairing symmetry is also C$_6$ symmetric.

In the second case we consider the $t$-$J$-$U$-$V$ model which corresponds to the main result

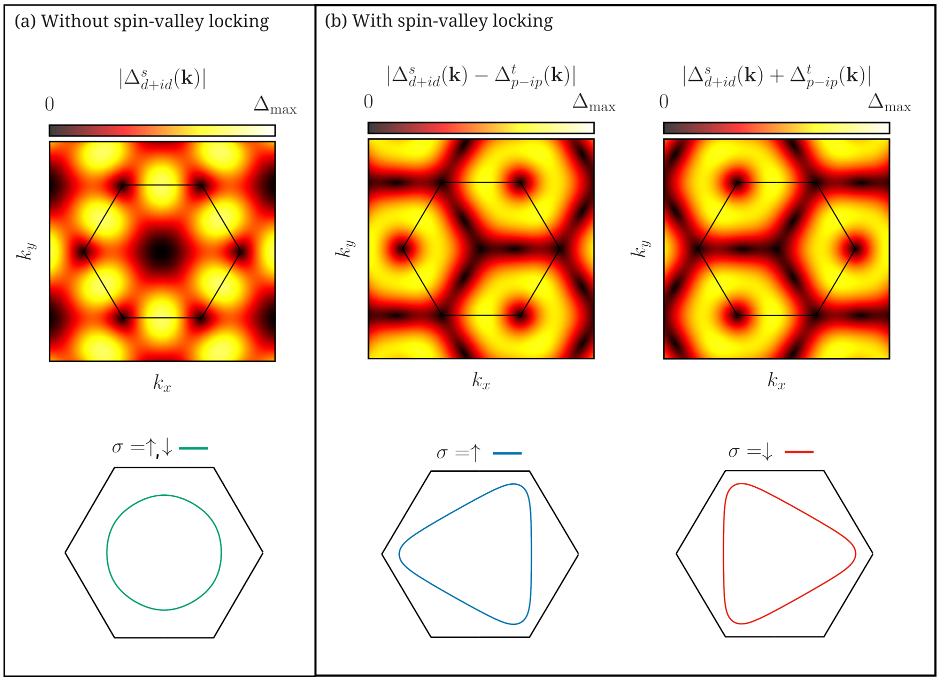


FIG. S5. The **k**-dependent SC gaps and the normal-state Fermi surfaces for two cases: (a) $t$-$J$-$U$ model when the Ising-type spin orbit coupling is absent and consequently there is no spin-valley locking (triangular lattice with purely real hoppings conserving $C_6$ symmetry); (b) $t$-$J$-$U$-$V$ model when the Ising type spin-orbit coupling is present leading to spin-valley locking (triangular lattice with spin dependent complex hoppings conserving $C_3$ symmetry). Both cases correspond to $n = 1$, $|t| = 8.27$ meV, $U = 80$ meV, $J = 4t^2/U$. Additionally for (b) we take $V = 22$ meV and $D = 0.3$ V/nm. In the lower part of the panel the Fermi surfaces are shown. Note that in the mixed singlet-triplet state considered in (b) there are two different SC gap distributions realized in **k**-space [cf. Eq. (S16)] in contrast to the situation with pure singlet pairing in (a).

from our manuscript (Fig. 2e of the manuscript), where the SOC is taken into account. Here we take $D = 0.3$ V/nm which corresponds to relatively large values of the SC amplitude in the diagram provided in Fig. 2e of the manuscript. Now the hoppings are complex are spin dependent with the form factor $\phi \approx 7\pi/8$. Due to the presence of the spin-valley locking the $C_6$ symmetry is broken and we are left with a $C_3$ symmetry and two separate Fermi surfaces; one for spin-up and $K'$ valley, one for spin-down and $K$ valley, as shown in Fig. S5(b). According to our calculations, for this case a stable SC solution corresponds to a mixed $d + id$ and $p - ip$ symmetry of the gap. As one can see in Fig. S5(b) this particular composition of the symmetry components leads to a situation in which the SC gap fulfills

the $C_3$ symmetry. Moreover, there are two different SC gap distributions realized in $\mathbf{k}$-space [cf. Eq. (S16)] in contrast to the situation with pure singlet pairing in (a). This allows for the SC gap to adjust to the shape of the two separate Fermi surfaces resulting from the spin-valley locking. Therefore, the mixed symmetry of the gap is a straightforward result of the spin-valley locking which leads to reduction of the symmetry from $C_6$ to $C_3$ and to two separate Fermi surfaces.

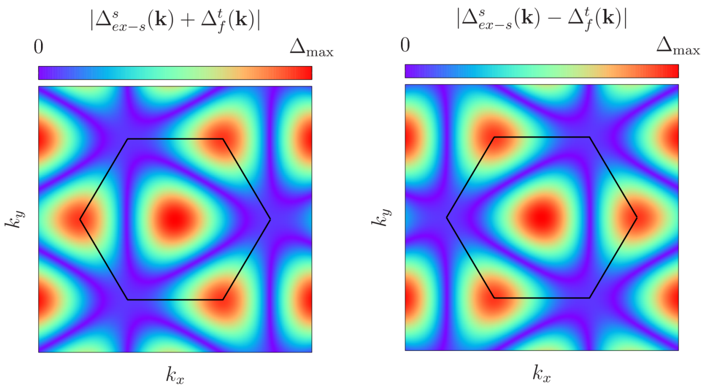


FIG. S6. The $\mathbf{k}$-dependent SC gaps for the case of *extended* $s/f$ mixed state which becomes stable in the low- ($n \approx 0$) and high- ($n \approx 2$) electron concentration regimes and requires $V \approx 0$ and/or high values of $J$.

The obtained mixed $d+id/p-ip$ state leads to the same free energy as the $d-id/p+ip$ state. Therefore, similarly as in the case of the pure $d \pm id$ pairing in the absence of the spin-valley locking, also here we have a degeneracy. Another pairing channel which is possible in the considered system is a mixed *extended s-wave* and *f-wave* state (cf. Fig. S6). However, it is much more fragile and appears only for the $V = 0$ case and/or for larger values of $J$. If those conditions are met and *extended s-wave*/*f-wave* state becomes stable for the band fillings close to the empty and fully filled situations. As one can see from Fig. S6 in this case a significant SC gap can be opened if the Fermi surfaces are relatively small and located at the $\Gamma$ point or the $K$ and $K'$ points of the Brillouin zone. Such situation appears for very low and very high electron concentrations which is not the case considered in our manuscript since we focus on $n \in [0.8, 1.2]$.

It should be emphasized that in the obtained mixed state, the opposite signs of the imaginary part in the $d \pm id$ and $p \mp ip$ amplitudes are of crucial importance. Only in such

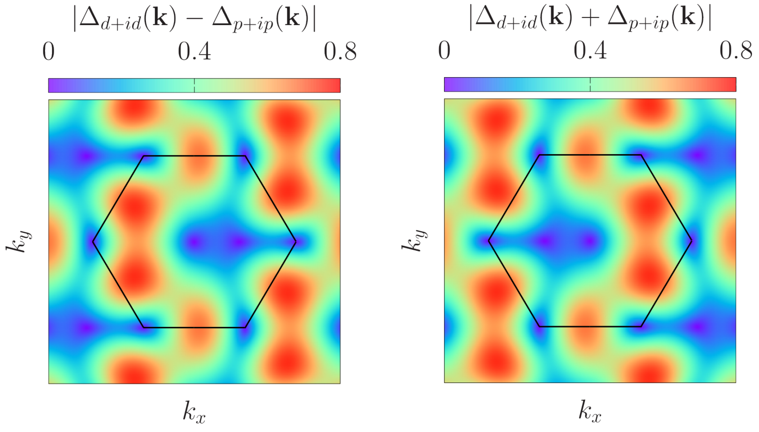


FIG. S7. The **k**-dependent SC gaps for the case of hypothetical $d + id/p + ip$ mixed state. As one can see in such case $C_2$ symmetry is realized not the $C_3$ which corresponds to our system with spin-valley locking. Therefore, such pairing channel is not likely to be realized here. The presented distributions have been obtained by setting the amplitudes $\Delta^s_{d+id} = 1$ and $\Delta^t_{p+ip} = 0.5$ and correspond to a representative situation.

case can one obtain an SC gap which realizes the $C_3$ symmetry resulting from the spin-valley locking. For the sake of clarity, in Fig. S7 we show the **k**-dependence of the SC gap for a hypothetical mixed $d + id/p + ip$ state which is not a result of self-consistent calculations but has been determined by assuming $\Delta^s_{d+id} = 1$ and $\Delta^s_{p+ip} = 0.5$. As one can see here, a $C_2$ symmetry is realized. Stabilization of such a state would require some additional symmetry breaking, which is not energetically favorable according to our calculations.

It should be noted that instabilities towards mixed singlet-triplet pairing of $d/p$- as well as *extended* $s/f$- type have been also reported by using functional renormalization group (FRG) [22, 23] as well as density matrix renormalization group (DMRG) [24] methods for the case of $tWSe_2$ within a single- and three- band pictures. Moreover, recent studies carried out within the continuum model have shown that for non-zero displacement field, the leading pairing instability corresponds to the two-dimensional $E$ representation which similarly gives rise to a chiral mixed singlet/triplet superconducting channels in large regime of parameters [25, 26]. However, in contrast to our results, Ref. [25] shows a transition to a time-reversal symmetric nematic state at high values of displacement field. Such transition might originate from the details of the continuum model which are not captured by the effective single-band approach taken here. Nevertheless, according to the experimental data,

the SC state is contained in a relatively small range of band fillings and displacement fields. Therefore, it is not completely clear if the regime of large $D$ values at which the transition to the namatic phase could appear according to Ref. [25], is reached.

Finally, apart from the symmetry related aspect, the effect of the spin-valley locking on the paired state appears also via the density of states. Namely, as discussed in Section I, the displacement field tunes the spin-valley locking, which affects the location of the Van Hove singularity. As discussed in detail in the main part of the manuscript [cf Fig. 2(e,j) of the manuscript], the SC state is stabilized at the crossing between the Van Hove singularity and the half-filling. This is due to the fact, that high values of the density of states enhance superconductivity, and additionally half-filling provides large renormalization which also stabilizes pairing. The maximal pairing amplitudes and, therefore, the most stable SC state appear for $n \approx 1$ and $D \approx 0.3 - 0.35$ V/nm. As one can see in Fig. S5(b) which corresponds to this regime, the Fermi surfaces almost reach the $K$ and $K'$ points and the spin splitting is well pronounced. This is due to the fact that the Fermi energy is in the proximity of thee Van Hove singularity, hence, we are close to the transition point between the closed electron-like Fermi surfaces and opened hole-like Fermi surfaces.

## III. TOPOLOGICAL PROPERTIES

To identify the topological properties of the obtained paired state we have calculated the Chern number by using the the Brillouin zone triangulation method [27]. According to our calculations in the relevant range of parameters corresponding to Fig. 2(e,j) in the main text of the manuscript, the superconducting state is nontrivial topologically with the Chern number $C = \pm 4$. For clarity we revisit here the mentioned diagram slightly zoomed in Fig. S8. As one can see, the sign change of $C$ appears at the line representing the Van Hove singularity.

To analyze further the topological nature of the obtained paired state we consider two representative sets of parameters which are marked by green dots in Fig. S8(a). In Fig. S9 we provide the corresponding $\mathbf{k}$-dependent SC gap as well as the normal state Fermi surfaces. As one can see, there are points at which the SC gap closes which are called nodal points. Each nodal point carries a topological charge (Chern charge). The Chern number of the superconducting state is equal to the sum of the topological charge contained in the

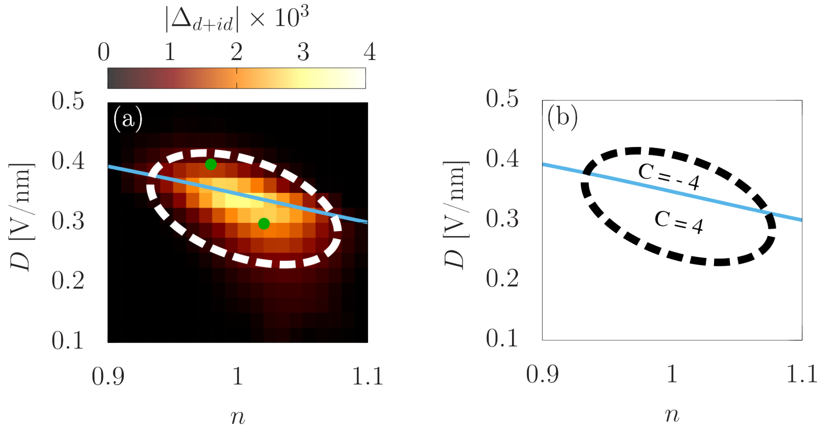


FIG. S8. (a) The SC gap amplitude as a function of band filling and displacement field for the case of $U = 80$ meV, $J = 4t^2/U$, $V = 22$ meV (the same model parameters as in Fig. 2e in the main text of the manuscript). Here we provide only the $d + id$ singlet component since the triplet one shows the same behavior but is approximately twice smaller. The white dashed line is a guide to the eye denoting the stability range of the SC state. The two green points correspond to the two representative $n$ and $D$ values leading to $C = \pm 4$ and selected for the detailed analysis of the topological features provided on Fig. S9. (b) The phase diagram which shows the calculated values of the Chern number characterizing the obtained superconducting state.

normal-state Fermi surface. Namely,

$$C = \sum_{i \in \Omega_{FS}} (-1)^w C_i, \tag{S20}$$

where $C_i$ is the topological charge of a given nodal point which can be determined by calculating the winding number of the order parameter around it. The sign of the Chern charge depends on whether it is enclosed by an electron- ($w = 0$) or hole-like ($w = 1$) Fermi surface. The $i$ index runs only over the nodal points that are contained inside the Fermi surface.

As one can see, the spin up and spin down Fermi surfaces introduce the Chern number equal $\pm 2$ each, which in total gives $\pm 4$. Moreover, the positive (negative) Chern number corresponds to electron-like (hole-like) Fermi surfaces centered at $\Gamma$ point ($K$ and $K'$ points). That is why the sign change of the Chern number in the diagram presented in Fig. S8(b) appears at the line representing the Van Hove singularity. As discussed in detail in Section I, the Van Hove singularity line represents the transition between the electron-like and hole-like

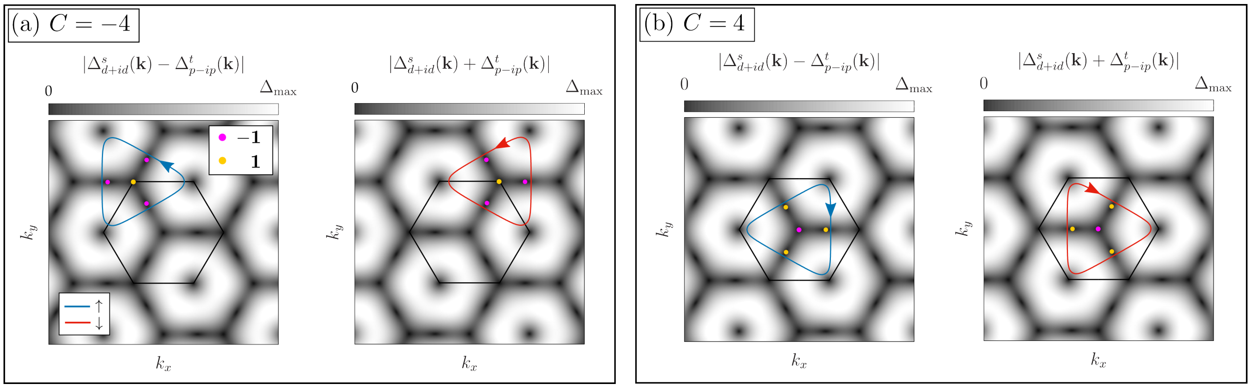


FIG. S9. The normal-state Fermi surfaces for spin-up and -down (blue and red solid lines) electrons as well as the **k**-dependent SC gaps for two selected values of $n$ and $D$, which are marked by green dots in Fig. S8 and correspond to following values of the Chern number: $C = -4$ (a), $C = 4$ (b). Note, that the value of the Chern number is simply the sum of the Chern charges contained inside the spin-up and -down Fermi surfaces (marked by the colored dots). The arrows at the Fermi surfaces represent the winding direction which is counterclockwise (clockwise) for the electron-like (hole-like) Fermi surfaces. Note that the signs of the Chern charges depend on the winding direction.

Fermi surfaces, which, as shown here, also leads to sign change of the Chern number.

---


[1] L. Wang, E.-M. Shih, A. Ghiotto, L. Xian, D. A. Rhodes, C. Tan, M. Claassen, D. M. Kennes, Y. Bai, B. Kim, K. Watanabe, T. Taniguchi, X. Zhu, J. Hone, A. Rubio, and C. R. Pasupathy, Abhay N. amd Dean, Correlated electronic phases in twisted bilayer transition metal dichalcogenides, Nature Materials **19**, 861 (2020).

[2] D. Xiao, G.-B. Liu, W. Feng, X. Xu, and W. Yao, Coupled spin and valley physics in monolayers of mos$_2$ and other group-vi dichalcogenides, Phys. Rev. Lett. **108**, 196802 (2012).

[3] Y. Zhang, L. Li, J.-H. Sun, D.-H. Xu, R. Lü, H.-G. Luo, and W.-Q. Chen, Kondo effect in monolayer transition metal dichalcogenide ising superconductors, Phys. Rev. B **101**, 035124 (2020).

[4] H. Pan, F. Wu, and S. Das Sarma, Band topology, hubbard model, heisenberg model, and dzyaloshinskii-moriya interaction in twisted bilayer wse$_2$, Phys. Rev. Res. **2**, 033087 (2020).

[5] Y.-T. Hsu, F. Wu, and S. Das Sarma, Spin-valley locked instabilities in moiré transition metal

dichalcogenides with conventional and higher-order van hove singularities, Phys. Rev. B **104**, 195134 (2021).

[6] J. Zang, J. Wang, J. Cano, and A. J. Millis, Hartree-fock study of the moiré hubbard model for twisted bilayer transition metal dichalcogenides, Phys. Rev. B **104**, 075150 (2021).

[7] M. Bélanger, J. Fournier, and D. Sénéchal, Superconductivity in the twisted bilayer transition metal dichalcogenide wse$_2$: A quantum cluster study, Phys. Rev. B **106**, 235135 (2022).

[8] J. Zang, J. Wang, J. Cano, A. Georges, and A. J. Millis, Dynamical mean-field theory of moiré bilayer transition metal dichalcogenides: Phase diagram, resistivity, and quantum criticality, Phys. Rev. X **12**, 021064 (2022).

[9] F. Wu, T. Lovorn, E. Tutuc, and A. H. MacDonald, Hubbard model physics in transition metal dichalcogenide moiré bands, Phys. Rev. Lett. **121**, 026402 (2018).

[10] Y. and D. N. Sheng, Topological chiral and nematic superconductivity by doping mott insulators on triangular lattice, Phys. Rev. X **12**, 031009 (2022).

[11] S. Daul, D. J. Scalapino, and S. R. White, Pairing correlations on $t - U - J$ ladders, Phys. Rev. Lett. **84**, 4188 (2000).

[12] S. Basu, R. J. Gooding, and P. W. Leung, Enhanced bound-state formation in two dimensions via stripelike hopping anisotropies, Phys. Rev. B **63**, 100506 (2001).

[13] E. Plekhanov, S. Sorella, and M. Fabrizio, Increasing $d$-wave superconductivity by on-site repulsion, Phys. Rev. Lett. **90**, 187004 (2003).

[14] T. Xiang, H. G. Luo, D. H. Lu, K. M. Shen, and Z. X. Shen, Intrinsic electron and hole bands in electron-doped cuprate superconductors, Phys. Rev. B **79**, 014524 (2009).

[15] M. Abram, J. Kaczmarczyk, J. Jędrak, and J. Spałek, $d$-wave superconductivity and its coexistence with antiferromagnetism in the $t$–$j$–$u$ model: Statistically consistent gutzwiller approach, Phys. Rev. B **88**, 094502 (2013).

[16] R. B. Laughlin, Gossamer superconductivity (2002), arXiv:cond-mat/0209269 [cond-mat.supr-con].

[17] F. C. Zhang, Gossamer superconductor, mott insulator, and resonating valence bond state in correlated electron systems, Phys. Rev. Lett. **90**, 207002 (2003).

[18] J. Spałek, M. Zegrodnik, and J. Kaczmarczyk, Universal properties of high-temperature superconductors from real-space pairing: $t - j - u$ model and its quantitative comparison with experiment, Phys. Rev. B **95**, 024506 (2017).

[19] J. Bünemann, T. Schickling, and F. Gebhard, Variational study of fermi surface deformations in hubbard models, Europhysics Letters **98**, 27006 (2012).

[20] J. Spałek, M. Fidrysiak, M. Zegrodnik, and A. Biborski, Superconductivity in high-tc and related strongly correlated systems from variational perspective: Beyond mean field theory, Physics Reports **959**, 1 (2022).

[21] J. Kaczmarczyk, Comparison of two approaches for the treatment of gutzwiller variational wave functions, Philosophical Magazine **95**, 563 (2015), https://doi.org/10.1080/14786435.2014.965235.

[22] L. Klebl, A. Fischer, L. Classen, M. M. Scherer, and D. M. Kennes, Competition of density waves and superconductivity in twisted tungsten diselenide, Phys. Rev. Res. **5**, L012034 (2023).

[23] A. Fischer, L. Klebl, V. Crépel, S. Ryee, A. Rubio, L. Xian, T. O. Wehling, A. Georges, D. M. Kennes, and A. J. Millis, Theory of intervalley-coherent afm order and topological superconductivity in twse$_2$ (2024), arXiv:2412.14296 [cond-mat.str-el].

[24] F. Chen and D. N. Sheng, Singlet, triplet, and pair density wave superconductivity in the doped triangular-lattice moiré system, Phys. Rev. B **108**, L201110 (2023).

[25] D. Guerci, D. Kaplan, J. Ingham, J. H. Pixley, and A. J. Millis, Topological superconductivity from repulsive interactions in twisted wse$_2$ (2024), arXiv:2408.16075 [cond-mat.supr-con].

[26] C. Schrade and L. Fu, Nematic, chiral and topological superconductivity in transition metal dichalcogenides (2024).

[27] T. Fukui, Y. Hatsugai, and H. Suzuki, Chern numbers in discretized brillouin zone: Efficient method of computing (spin) hall conductances, Journal of the Physical Society of Japan **74**, 1674 (2005), https://doi.org/10.1143/JPSJ.74.1674.
